# Supplementary material for: Contract-Based Cooperative Spectrum Sharing
Source: arXiv:1102.4176 source file (2011-02-21)
Supplement: Supplementary file 1 [file Appendix.tex]

%!TEX root = main.tex
%SourceDoc main.tex

\appendix

\subsection{Proof of Theorem \ref{prop:suff}}
\label{proof:thm1}

\subsubsection{Proof of sufficient conditions}

We use mathematical induction to prove this proposition. Let us denote
$\Phi(n)$ as a subset which contains the first $n$
power-time combinations in the complete contract $\Phi$ (i.e.,
$\Phi(n)=\{(p_k,t_k),|k=1,...,n\}$).

We first show that $\Phi(1)$ is feasible. Since there is only one SU
type, the contract is feasible if it satisfies IR constraint in
(\ref{eq:IR}). This is true due to $\mathtt{Contd.b}$ in
Proposition~\ref{prop:suff}.

We next show that if contract $\Phi(k)$ is feasible, then we can
construct the new contract $\Phi(k+1)$ by adding new item
$(p_{k+1},t_{k+1})$ and show that the new contract is also feasible. To achieve
this, we need to show two results:
\begin{itemize}
\item \emph{Result I:} the IC
and IR constraints for type-$\theta_{k+1}$ SUs:
\begin{equation}%\label{eq:add_k+1}
\begin{cases} \; \theta_{k+1}t_{k+1}-p_{k+1}\geq \theta_{k+1}t_i-p_i,\ \forall
i=1,...,k\\
\; \theta_{k+1}t_{k+1}-p_{k+1}\geq 0,
\end{cases}\nonumber(27)
\end{equation}
\item \emph{Result II:} for types $\theta_1,...,\theta_k$ already contained in the contract $\Phi(k)$, the IC constraints
are still satisfied after adding the new type $\theta_{k+1}$:
\begin{equation}%\label{eq:add_k+1_original}
\ \ \ \ \ \ \ \ \ \theta_it_i-p_i\geq \theta_it_{k+1}-p_{k+1},
\forall i=1,...,k.\ \ \ \ \ \ \ \nonumber(28)
\end{equation}
Note that the new contract $\Phi(k+1)$ will satisfy the IR
constraints of all type $\theta_1$ to $\theta_k$ SUs as the original
contract $\Phi(k)$ is feasible.
\end{itemize}
%there is no need to check the IR constraints for original
%types after introducing a new type, because original SUs'
%non-negative payoffs sticking to their original type items will not
%change.

\emph{Proof of Result I in (27):} First, we prove the IC constraint
for type $\theta_{k+1}$. Since contract $\Phi(k)$ is feasible, the
IC constraint for a type-$\theta_i$ SU must hold, i.e.,
$$\theta_kt_i-p_i\leq \theta_kt_k-p_k, \forall i=1,...,k.$$ Also,
the right inequality of (\ref{eq:contdc}) in $\mathtt{Contd.c}$ can
be transformed to
$$p_{k+1}\leq p_k+\theta_{k+1}(t_{k+1}-t_k).$$
By combining the
above two inequalities, we have
\begin{equation}%\label{eq:proof_I}
\theta_kt_i-p_i+p_{k+1}\leq
\theta_kt_k+\theta_{k+1}(t_{k+1}-t_k),\forall i=1,...,k.\
\nonumber(29)
\end{equation}
Notice that $\theta_{k+1}>\theta_k$ and $t_k\geq t_i$ in
$\mathtt{Contd.a}$. We also have
$$\theta_{k+1}t_k-\theta_{k+1}t_i\geq \theta_kt_k-\theta_kt_i.$$
By substituting this inequality into (29), we have
\begin{equation}%\label{eq:appendix_1}
\ \ \ \ \ \ \ \ \  \ \ \ \ \theta_{k+1}t_{k+1}-p_{k+1}\geq
\theta_{k+1}t_i-p_i,\ \ \ \ \ \ \ \ \ \ \ \ \ \ \ \ \ \ \ \
\nonumber (30)\end{equation} which is actually the IC constraint for
type $\theta_{k+1}$.

Next, we show the IR constraint for type $\theta_{k+1}$. Since
$\theta_{k+1}>\theta_i$ for any $i\leq k$, then
$$\theta_{k+1}t_i-p_i>\theta_it_i-p_i.$$
Using (30), we also have
$$\theta_{k+1}t_{k+1}-p_{k+1}\geq \theta_{k+1}t_i-p_i.$$
By combining the last two inequalities, we have
$$\theta_{k+1}t_{k+1}-p_{k+1}\geq 0,$$
which proves the IR constraint.
%
%Due to IC constraint for type $\theta_{k+1}$ which we just proved,
%we have
%$$\theta_{k+1}t_{k+1}-p_{k+1}\geq \theta_{k+1}t_i-p_i,\forall i=1,...,k.$$
%we can further derive
%$$\theta_{k+1}t_{k+1}-p_{k+1}\geq \theta_it_i-p_i,$$
%where the right-hand side expression is non-negative due to IR
%constraint of type $\theta_i$ in the feasible contract $\Phi(k)$.

\emph{Proof of Result II in (28):} Since contract $\Phi(k)$ is
feasible, the IC constraint for type $\theta_i$ holds, i.e.,
$$\theta_it_k-p_k\leq \theta_it_i-p_i, \forall i=1,...,k.$$
Also, we can transform the left inequality of (\ref{eq:contdc}) in
$\mathtt{Contd.c}$ to
$$p_k+\theta_k(t_{k+1}-t_k)\leq p_{k+1}.$$
By combining the above two inequalities, we conclude
\begin{equation}%\label{eq:proof_II}
\ \ \ \ \ \ \ \ \ \ \theta_it_k+\theta_k(t_{k+1}-t_k)\leq
\theta_it_i-p_i+p_{k+1}.\ \ \ \ \ \ \ \ \ \nonumber(31)
\end{equation}
Note that $\theta_k\geq \theta_i$ for any $i\leq k$ and $t_{k+1}\geq
t_k$ in $\mathtt{Contd.a}$. We also have
$$\theta_kt_{k+1}-\theta_kt_k\geq \theta_it_{k+1}-\theta_it_k.$$
By combining the above two inequalities, we conclude
$$\theta_it_{k+1}-p_{k+1}\leq \theta_it_{i}-p_i, \forall i=1,\ldots, k$$
which is actually the IC constraint for type $\theta_i$.

\subsubsection{Proof of necessary conditions}
It is easy to check
that the sufficient conditions in Proposition~\ref{prop:suff} are
also necessary for a feasible contract. Specifically,
$\mathtt{Contd.a}$ is the same as necessary conditions summarized in
(\ref{eq:neccessary}). $\mathtt{Contd.b}$ is same as the necessary
IR constraint for the lowest type $\theta_1$ in a feasible contract.
The left inequality of $\mathtt{Contd.c}$ can be derived from the
necessary IC constraint for type $\theta_{k-1}$ in a feasible
contract, and the right inequality of $\mathtt{Contd.c}$ can also be
derived from the necessary IC constraint for type $\theta_k$.
%Hence,
%Proposition~\ref{prop:suff} shows both the sufficient and necessary
%conditions for a feasible contract.
\hfill$\rule{2mm}{2mm}$

\subsection{Proof of Proposition
\ref{prop:incomplete1}}\label{proof:prop}

First, it is
not difficult to check that the relay powers in
(\ref{eq:incomplete_power}) satisfy the sufficient conditions of
contract feasibility in Theorem~\ref{prop:suff}. We skip the details
here due to the page limit.

Next we prove the optimality and uniqueness of the solutions in
(\ref{eq:incomplete_power}).

\subsubsection{Proof of optimality}

We first show that the relay powers in (\ref{eq:incomplete_power})
maximize the PU's utility given fixed time allocations, i.e.,
$\{p_k^{\ast},\forall k\}$ maximize
\begin{equation}%\label{eq:incomplete_power_opt}
\ \ \ \ \
\frac{1}{1+\sum_{k\in\mathcal{K}}N_kt_k}(\frac{R^{dir}}{2}+\frac{1}{2}\log(1+\frac{\sum_{k\in\mathcal{K}}N_kp_k}{n_0})).\nonumber
\ \ \ \ \ (32)
\end{equation}
We prove by contradiction. Suppose that these exists another
feasible relay powers $\{\tilde{p}_k,\forall k\}$ which achieves a
better solution than $\{p_k^\ast,\forall k\}$ in
(\ref{eq:incomplete_power}). Since (32) is increasing in total relay
power, we must have
$\sum_{k\in\mathcal{K}}N_k\tilde{p}_k>\sum_{k\in\mathcal{K}}N_k{p_k^{\ast}}$.
Thus we have at least one relay power $\tilde{p}_k>p_k^{\ast}$ for
one type $\theta_k$.

If $k=1$, then $\tilde{p}_1>p_1^{\ast}$. Since
$p_1^{\ast}=\theta_1t_1$, then $\tilde{p}_1>\theta_1t_1$. But this
violates the IR constraint for type $\theta_1$. Then we must have
$k>1$.

Since $\{\tilde{p}_k,\forall k\}$ is feasible, then
$\{\tilde{p}_k,\forall k\}$ must satisfy the right inequality of
$\mathtt{Contd.c}$ in Theorem~\ref{prop:suff}. Thus we have
$$\tilde{p}_k\leq \tilde{p}_{k-1}+\theta_k(t_k-t_{k-1}).$$
By substituting $\theta_k(t_k-t_{k-1})=p_k^{\ast}-p_{k-1}^{\ast}$ as
in (\ref{eq:incomplete_power}) into the this inequality, we have
$$\tilde{p}_{k-1}>p_{k-1}^{\ast}.$$
Using the above argument repeatedly, we finally obtain that
$$\tilde{p}_1>p_1^{\ast}=\theta_1t_1,$$
which violates the IR constraint for type-$\theta_1$ again.

\subsubsection{Proof of uniqueness}

We next prove that the relay powers in (\ref{eq:incomplete_power})
is the unique solution that maximizes (32). We also prove by
contradiction. Suppose that there exists another
$\{\bar{p_k},\forall k\}\neq \{p_k^{\ast},\forall k\}$ such that
$\sum_{k\in\mathcal{K}}N_k\bar{p}_k=\sum_{k\in\mathcal{K}}N_k{p_k^{\ast}}$
in (32). Then there is at least one relay power
$\bar{p}_i<p_i^{\ast}$ and one relay power $\bar{p}_j>p_j^{\ast}$.
We can focus on type-$\theta_j$ and $\bar{p}_j>p_j^{\ast}$. By using
the same argument before, we have
$\bar{p}_1>p_1^{\ast}=\theta_1t_1$. But this violates the IR
constraint for type $\theta_1$. \hfill$\rule{2mm}{2mm}$

\subsection{Proof of
Theorem~\ref{thm:incomplete1}}\label{proof:incomplete1}
\emph{Proof.} We prove by contradiction. Suppose that there exists
an optimal contract item with $t_k>0$ for the type-$\theta_k$ SUs
with $k<K$. The total time allocation is
$T'=\sum_{k\in\mathcal{K}}N_kt_k$ in this case. Then PU's utility is
\begin{equation}%\label{eq:incomplete1_proof1}
u_{PU}^1=\frac{\frac{R^{dir}}{2}+\frac{1}{2}\log\left(1+\frac{\sum_{k\in\mathcal{K}}N_k(\theta_1t_1+\sum_{i=2}^k\theta_i(t_i-t_{i-1}))}{n_0}\right)}{1+T'}.\nonumber
(33)
\end{equation}
Next we show that given a fixed total time allocation $T'$,
allocating positive time only to the highest type SUs (i.e.,
$N_Kt_K=T'$) achieves a larger utility for the PU as follows
\begin{equation}%\label{eq:incomplete_proof2}
\ \ \ \ \ \ \ \ \ \ \ \
u_{PU}^2=\frac{\frac{R^{dir}}{2}+\frac{1}{2}\log\left(1+\frac{\theta_KN_Kt_K}{n_0}\right)}{1+T'}.\nonumber
\ \ \ \ \ \ \ \ \ \ \ \ \ (34)
\end{equation}
This is because $\theta_KN_Kt_K=\theta_KT'$ in (34) and
$$\sum_{k\in\mathcal{K}}N_k(\theta_1t_1+\sum_{i=2}^k\theta_i(t_i-t_{i-1}))<\theta_KT'$$
in (33), thus (34) is larger than (33). This contradicts with the
optimality of the contract, and thus we completes the proof.
\hfill$\rule{2mm}{2mm}$

%%%%%%%
\subsection{Proof of Proposition
\ref{prop:incomplete2}}\label{proof:propincomplete2}

First, it is not difficult to check that the relay powers in (25)
satisfy the sufficient conditions of contract feasibility in
Theorem~\ref{prop:suff}.

Next we prove the optimality of the solutions in (25).

\subsubsection{Proof of optimality}

We first show that the relay powers in (25) maximize the PU's
expected utility given fixed time allocations, i.e.,
$\{p_k^{\ast},\forall k\}$ is the solution to (24).
%maximize
%\begin{equation}\label{eq:incomplete_power_opt}
%\frac{1}{1+\sum_{k\in\mathcal{K}}N_kt_k}(\frac{R^{dir}}{2}+\frac{1}{2}\log(1+\frac{\sum_{k\in\mathcal{K}}N_kp_k}{n_0})).
%\end{equation}
We prove by contradiction. Suppose that these exists another
feasible relay powers $\{\tilde{p}_k,\forall k\}$ which achieves a
better solution than $\{p_k^\ast,\forall k\}$ in (25). Since PU's
expected utility in (24) is increasing in total relay power, we must
have
$\sum_{k\in\mathcal{K}}N_k\tilde{p}_k>\sum_{k\in\mathcal{K}}N_k{p_k^{\ast}}$.
Thus we have at least one relay power $\tilde{p}_k>p_k^{\ast}$ for
one type $\theta_k$.

If $k=1$, then $\tilde{p}_1>p_1^{\ast}$. Since
$p_1^{\ast}=\theta_1t_1$, then $\tilde{p}_1>\theta_1t_1$. But this
violates the IR constraint for type $\theta_1$. Then we must have
$k>1$.

Since $\{\tilde{p}_k,\forall k\}$ is feasible, then
$\{\tilde{p}_k,\forall k\}$ must satisfy the right inequality of
$\mathtt{Contd.c}$ in Theorem~\ref{prop:suff}. Thus we have
$$\tilde{p}_k\leq \tilde{p}_{k-1}+\theta_k(t_k-t_{k-1}).$$
By substituting $\theta_k(t_k-t_{k-1})=p_k^{\ast}-p_{k-1}^{\ast}$ as
in (25) into the this inequality, we have
$$\tilde{p}_{k-1}>p_{k-1}^{\ast}.$$
Using the above argument repeatedly, we finally obtain that
$$\tilde{p}_1>p_1^{\ast}=\theta_1t_1,$$
which violates the IR constraint for type-$\theta_1$ again.

\subsubsection{Proof of uniqueness}

We next prove that the relay powers in (25) is the unique solution
that maximizes (24). We also prove by contradiction. Suppose that
there exists another $\{\bar{p_k},\forall k\}\neq
\{p_k^{\ast},\forall k\}$ such that
$\sum_{k\in\mathcal{K}}N_k\bar{p}_k=\sum_{k\in\mathcal{K}}N_k{p_k^{\ast}}$
in (24). Then there is at least one relay power
$\bar{p}_i<p_i^{\ast}$ and one relay power $\bar{p}_j>p_j^{\ast}$.
We can focus on type-$\theta_j$ and $\bar{p}_j>p_j^{\ast}$. By using
the same argument before, we have
$\bar{p}_1>p_1^{\ast}=\theta_1t_1$. But this violates the IR
constraint for type $\theta_1$. \hfill$\rule{2mm}{2mm}$

\subsection{Proof of Observation \ref{ob:PU_time_DT} for $R^{dir}=0$}\label{proof:ob}
\emph{Proof.} When $R^{dir}=0$, the PU will always allocate positive
time to the highest type SUs (i.e., $t_K^\ast>0$). Its total time
allocation is decreasing in the highest type $\theta_K$. PU's
utility in (\ref{eq:incomplete_optimization2}) can be written as
\begin{equation}%\label{eq:ob_proof}
\ \ \ \ \ \ \
u_{PU}(t_K)=\frac{1}{2(1+N_Kt_K)}\log(1+\theta_KN_Kt_K).\nonumber\ \
\ \ \ \ (35)
\end{equation}
Denote the total time allocation to SUs as $T'$. We can rewrite (35)
as a function of $T'$:
%\begin{equation}
$$u_{PU}(T')=\frac{1}{2(1+T')}\log(1+\theta_KT'),$$
%\end{equation}
which can be shown as a concave function of $T'$. Since
$t_K^\ast>0$, we conclude that the optimal $T'^\ast=N_Kt_K\ast>0$
and satisfies
$$\frac{d u_{PU}(T')}{dT'}\mid_{T'=T'^\ast}=\frac{\frac{\theta_K(1+T'^\ast)}{1+\theta_KT'^\ast}-\log(1+\theta_KT'^\ast)}{2(1+T'^\ast)^2}=0,$$
i.e., \begin{equation}%\label{eq:ob_proof2}
F(\theta_K,T'^\ast):=\theta_K(1+T'^\ast)-(1+\theta_KT'^\ast)\log(1+\theta_KT'^\ast)=0.\nonumber
(36)
\end{equation}
Since
$$\frac{\partial F(\theta_K,T'^\ast)}{\partial \theta_K}=1-T'^\ast\log(1+\theta_KT'^\ast),
$$
$$\frac{\partial F(\theta_K,T'^\ast)}{\partial
T'^\ast}=-\theta_K\log(1+\theta_KT'^\ast),$$ thus
\begin{equation}%\label{eq:ob_proof3}
\ \ \ \ \ \ \ \frac{dT'^\ast}{d\theta_K}=-\frac{\partial F/\partial
\theta_K}{\partial F/\partial
T'^\ast}=\frac{1-T'^\ast\log(1+\theta_KT'^\ast)}{\theta_K\log(1+\theta_KT'^\ast)}.\
\ \ \ \ \ \ \ \nonumber(37)
\end{equation}
Since $\theta_KT'^\ast>0$, we have
$$\log(1+\theta_KT'^\ast)-\theta_KT'^\ast<0.$$
By substituting this inequality into (36), we conclude
$$1-T'^\ast\log(1+\theta_KT'^\ast)<0,$$ and thus
$\frac{dT'^\ast}{d\theta_K}$ in (37) is negative. Hence, the optimal
total time allocation $T'^\ast$ is decreasing in the highest type
$\theta_K$. \hfill$\rule{2mm}{2mm}$
